# Supplementary material for: Irreducible decompositions of tensors via the Brauer algebra and applications to metric-affine gravity
Source: arXiv:2407.18019 source file (2024-07-25)
Supplement: Supplementary file 1 [file appendix2.tex]

%*************************************************
%*************************************************
\chapter{Mathematica Packages}
%*************************************************
%*************************************************

\section{SymmetricFunctions : }

\section{BrauerAlgebra : }

\section{xBrauer : }

\section{xMAG : }
